# Supplementary material for: Debiased inference for proximal dose-response function
Source: arXiv:2608.00404 source file (2026-10-07)
Supplement: Supplementary file 1 [file JASA-supp.tex]

\documentclass[12pt,letterpaper]{article}
\def\blind{0} % 0 = anonymous; 1 = with authors
\def\documentpart{2} % 0 = full; 1 = main; 2 = supplement
\input{document-driver}
